# Supplementary material for: Differentially Private Learning Needs Hidden State (Or Much Faster Convergence)
Source: arXiv:2203.05363 source file (2022-10-17)
Supplement: Supplementary file 1 [file append_pseudocode_mBGD.tex]

\begin{algorithm}[ht]
	\caption{$\algo_{\text{Noisy-mBGD}}$: Noisy mini-batch Gradient Descent}
	\label{alg:noisymBGD}
	\begin{algorithmic}
		\STATE {\bfseries Input:} Data domain $\X$. Dataset $\D = (\x_1, \x_2, \cdots, \x_\size)$ with $\x_i\in\Domain$. A convex parameter set $\C\subseteq\mathbb{R}^\dimension$ in Euclidean space. A loss function $\loss(\vtheta;\x)$ over $\C\times\X$ with gradient sensitivity $\lVert\nabla\ell(\theta,\x) - \nabla\ell(\theta,\x')\rVert_2\leq S_g$, learning rate schedule $\step_\kk^{j}$ and noise standard deviation schedule $\sig_\kk^{j}$ for $\kk=0, \cdots,\K-1$ and $j = 0, \cdots, n/b - 1$, parameter initialization $\vtheta_0$, mini-batch size $b$.
		\STATE{\bfseries Initialization:} $\theta_{0}^{0} = \theta_0$
		\FOR {$\kk = 0, 1, \cdots, \K - 1$}
		\STATE{\bfseries Batch generation:} form $n/b$ non-overlapping mini-batch subsets of $[n]$ with size $b$: $B_\kk^0, \cdots, B^{n/b-1}_\kk$.\label{step:batch_generation}
		\FOR {$j = 0, 1, \cdots, n/b - 1$}
		\STATE {$\g{\vtheta_{\kk}^{ j}}{\B^{j}_\kk}= \frac{1}{b}\sum_{x_\ii\in \B_\kk^{j}} \grad\loss(\vtheta_{\kk}^{j};\x_\ii)$}
		\STATE {$\vtheta_{\kk}^{j + 1} = \vtheta_{\kk}^{j} - \step_{\kk}^j\cdot \g{\vtheta_{\kk}^{j}}{\B_{\kk}^j} + \sqrt{2\step_\kk^j}\cdot \noise_{\kk}^j\cdot \Gauss{0}{\Id}$} \label{alg:ngd:updatestep}
		\ENDFOR
		\STATE {$\vtheta_{\kk + 1}^{0} = \vtheta_{\kk}^{n/b}$}
		\ENDFOR
		\STATE {Output $\vtheta_{\K}^{0}$}
	\end{algorithmic}
\end{algorithm}
